# Supplementary material for: Loss of memory of an elastic line on its way to limit cycles
Source: arXiv:2308.05603 ancillary file (2024-04-03)
Supplement: Supplementary file 1 [file SI.pdf]

# Loss of memory of an elastic line on its way to limit cycles – Supplementary Information

Elisabeth Agoritsas[1,*] and Jonathan Barés[2,†]

[1]Department of Quantum Matter Physics (DQMP), University of Geneva,
Quai Ernest-Ansermet 24, CH-1211 Geneva, Switzerland

[2]Laboratoire de Mécanique et Génie Civil (LMGC), UMR 5508 CNRS-University Montpellier, 34095 Montpellier, France

(Dated: April 2, 2024)

## CONTENTS

I. Detailed numerical recipe and parameters 1

II. Evolution of the velocity profiles towards the limit cycles 2

III. Memory characterisation: alternative criteria 2

IV. Link between, number of cycle $n$ and amnesia rate $s$ 3

V. Details about rescalings and partial data collapse 4

VI. Details about the amnesia phase diagram 4

VII. Continuous versus intermittent velocity dynamics 5

VIII. Typical case with periodic limit case 5

References 6

## I. DETAILED NUMERICAL RECIPE AND PARAMETERS

The numerical simulations consist in solving the evolution equation of the line/front $h(z,t)$ propagating in a quenched random field $\eta(x,z)$, with bi-periodic boundary conditions for $\{x,z\} \in [0,\ell] \times [0,N]$:

$$\zeta \partial_t h(z,t) = (ct - k \langle h(z,t) \rangle_z) + \frac{1}{\pi} \int_0^N \mathrm{d}z' \, \frac{h(z',t) - h(z,t)}{|z'-z|^\gamma} + \sigma \, \eta(h(z,t),z) \, . \tag{1}$$

Setting the friction coefficient to $\zeta = 1$ fixes the time units. The time evolution of $h(z,t)$ is obtained by solving this equation using a fourth-order Runge-Kutta scheme with a time discretisation of $10^{-3}$, as in [1–3]. The second right-hand term is obtained using a discrete Fourier transform along $z$ (periodic conditions along this axis). A discrete uncorrelated random Gaussian matrix of dimension $l \times N$, $\eta(x,z)$, is prescribed (with zero average and unit variance for each of its components). The third right-hand term is obtained via a linear interpolation of this matrix at $\{x',z\}$ with $x' = h(z,t) \pmod{l}$. At time $t=0$, the elastic line is a flat front $h(z,t=0)=0$.

Simulations are carried out for parameters: $\gamma = 2$, $c \in [10^{-5}, 5 \times 10^{-2}]$, $k \in [10^{-3}, 5 \times 10^{-1}]$, $\sigma \in [0.1, 5]$, and in pixel-size units $N \in [128, 16384]$, $l \in [2, 400]$. Depending on the variability of the measurement of the amnesia rate $s$, simulation for each family of parameters are repeated from 3 to 25 times for different disorder configurations; error-bars, when apparent, correspond to disorder sample-to-sample fluctuations.

For each simulation, the front shape $h(z,t)$ is saved each time $t_i$ when $\langle h(z,t_i) \rangle_z \pmod{l} = 0$. Because of the time discretisation, $h(z,t_i)$ is not determined exactly, a linear interpolation between two time steps is therefore used to approximate it very accurately. The simulation code is available upon request to the authors.

* elisabeth.agoritsas@unige.ch

† jonathan.bares@umontpellier.fr

## II. EVOLUTION OF THE VELOCITY PROFILES TOWARDS THE LIMIT CYCLES

In the main text, we describe how we quantify the convergence to a limit cycle, in a given disorder realisation of $\eta(x,z)$, by comparing consecutive cycles the profiles $h_j(z) \equiv h(z,t_j)$ and $v_j(z) \equiv \partial_t h(z,t_j)$. In Fig. 1 of the main text, we provide examples of the geometrical profile, here we provide in Fig. 1 the corresponding plots for the velocity profiles.

We first adapt the definitions of the stroboscopic snapshots to the velocity profiles:

$$\begin{aligned} \Delta v(z,t_{j+1},t_j) &\equiv v(z,t_{j+1}) - v(z,t_j), \\ \Delta v_j \equiv \langle \Delta v(z,t_{j+1},t_j) \rangle_z &= \frac{1}{N}\int_0^N \mathrm{d}z\, \Delta v(z,t_{j+1},t_j). \end{aligned} \tag{2}$$

In Fig. 1(a), we plot side by side the average difference $\Delta v_j$ and $\Delta h_j$, in order to follow how the line loses memory of its initial condition and eventually converges to a limit cycle, and what it means in terms of the velocity profiles. In Fig. 1(b)-(c), we plot the counterpart of Fig. 3(b)-(c) of the main text for the front speed at a specific point of the cycle ($x=0$) in the steady regime.

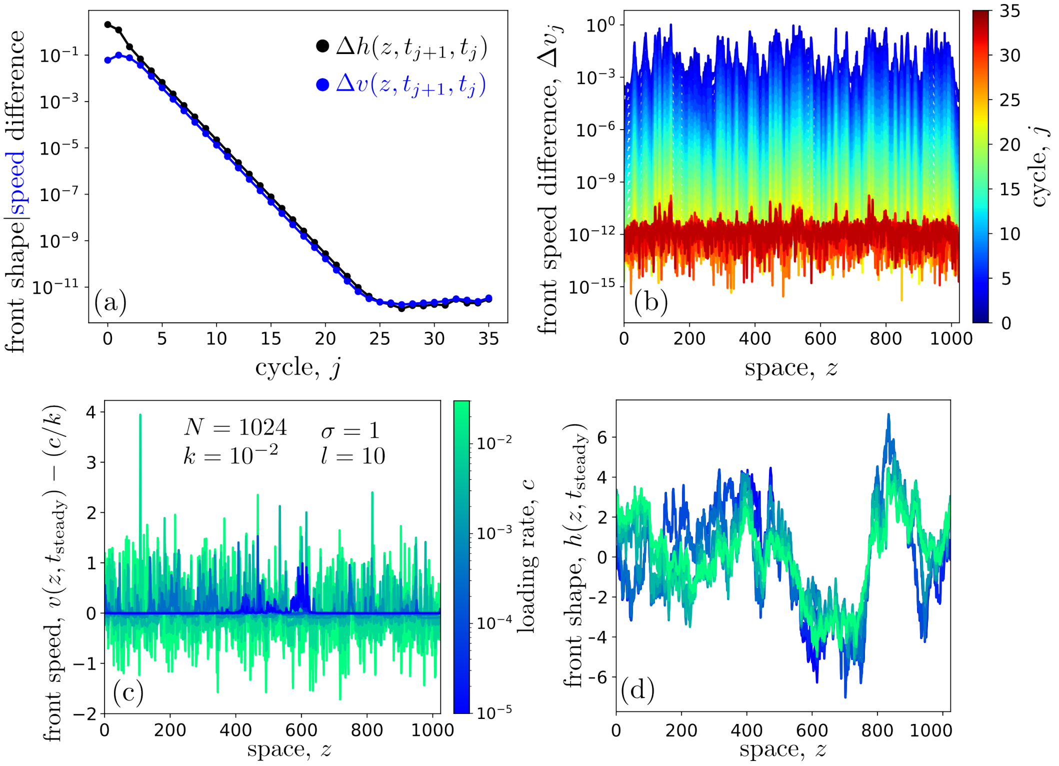


Figure 1. (a) Geometrical and velocity integrated profile differences, $\Delta h$ and $\Delta v$ respectively, as a function of the number of cycles. (b) Velocity profile difference, in absolute value, between successive cycles ($j$, $j+1$). (c) Front speed $v(z,t)$ when starting a new cycle in the converged regime ($t = t_{\mathrm{steady}}$) for increasing loading rate, for the same disorder and initial conditions. The speed profile is shifted from the average loading speed $c/k$. (d) Snapshots of the geometrical profiles when starting a new cycle, with the same color code and settings as in (c).

## III. MEMORY CHARACTERISATION: ALTERNATIVE CRITERIA

In the main text, the amnesia rate $s$ is measured from front different curves $\Delta h_j$ because it is the most straightforward and meaningful observable of the system, but different other strategies have been tested.

First, the activity map $M_m$ of each period $m$ can be calculated. It is a matrix of dimension $l \times N$, with each element $\{i,j\}$ giving the time spent by the front $\{z, h(z,t)\}$ in the pixel $[j, j+1] \times [i, i+1]$. To test if a front converges to a limit cycle, *i.e.* to the same way of crossing the disordered map, maps $M_m$ and $M_{m+1}$ are compared sequentially. The proxy for $\Delta h_m$ is then $\Delta M_m = \sum_{i,j} |M_m - M_{m+1}|$.

During the front propagation, several global signals $\bar{q}(x)$ are saved, for instance the spatially-averaged loading force, the spatially-averaged velocity, or even the stored elastic energy. Another proxy for $\Delta h_m$ is then to compare the evolution of these signals from one period to the next: $\Delta\bar{q}_m = \int_{lm}^{(l+1)m} dx' \, |\bar{q}(x') - \bar{q}(x'+l)|$.

These different criteria have been used to get the number of cycles $n$ for reaching amnesia. In Fig. 2 the number of cycles for amnesia as a function of the transverse size $\ell$ is plotted for the different measurement methods, for a given disorder configuration. We observe that whatever the method, results are consistent, supporting that we can safely focus on the most straightforward indicator, the evolution of the front difference, as reported in the main text.

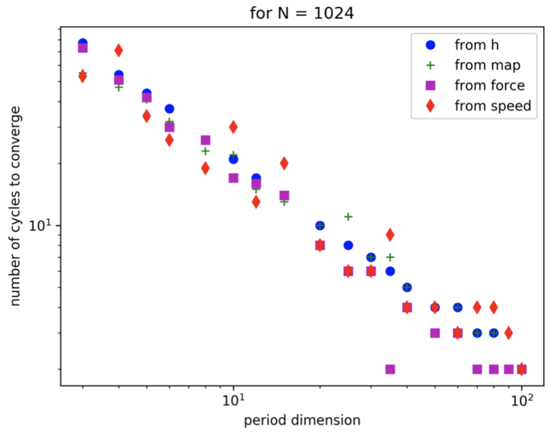


Figure 2. **Comparing alternative criteria**. Evolution of the number of cycles for amnesia $n$ with respect to the period dimension $l$ (other simulations parameters staying constant: $c = 10^{-3}$, $k = 10^{-2}$, $N = 1024$, $\sigma = 1$). $n$ is measured, respectively, via the front difference $h$ (as reported in the main text), via the activity map, via the averaged loading force, or via the average velocity.

## IV. LINK BETWEEN, NUMBER OF CYCLE $n$ AND AMNESIA RATE $s$

In the main text, even if the number of cycles for amnesia $n$ is more intuitive in order to explain the main mechanisms of the memory for the elastic line, for the sake of simplicity and accuracy of measurement we focused our analysis on the rate of amnesia $s$. As argued in the main text, the quantity $1/s$ is a good proxy for $n$. Here we illustrate and support this claim by plotting in Fig.3, for each set of parameters we have considered, $n$ *vs.* $1/s$ and we find indeed a linear relation.

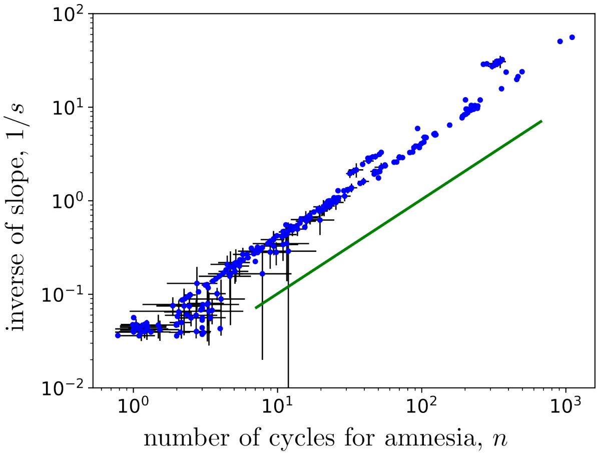


Figure 3. Number of cycles for amnesia ($n$) as a function of the inverse of the rate of amnesia ($1/s$), for each set of simulation parameters, we considered. Error-bars stand for different disorder realisations. The green line is a guide to the eye with a slope of 1.

## V. DETAILS ABOUT RESCALINGS AND PARTIAL DATA COLLAPSE

In the Fig. 2 of the main text, we present different partial rescalings, aiming at collapsing the **A** regime where memory is extensive. To further support the relevance of these scalings, in Fig. 4 we show the same figures with either no rescaling at all or with a single rescaling ($\sigma_{\text{eff}} = \sigma$ and $N_{\text{eff}} = N$, respectively).

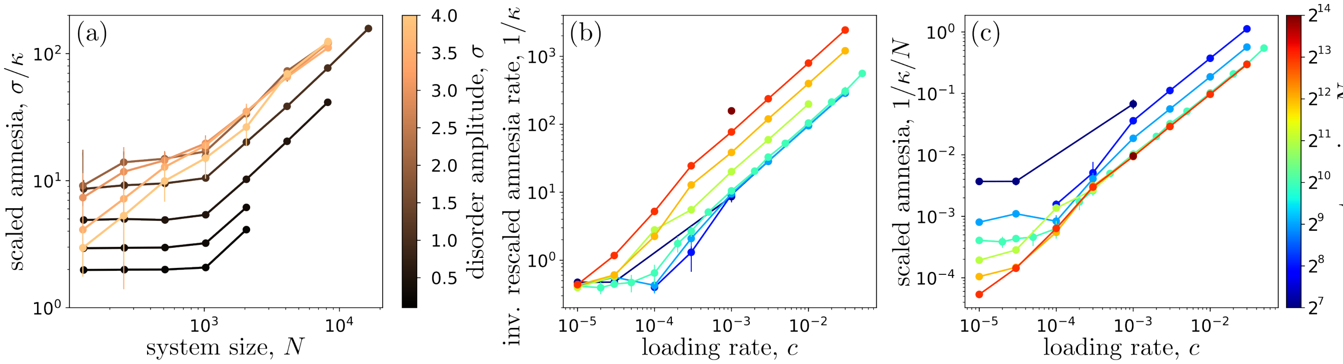


Figure 4. (a) Inverse of the rescaled amnesia rate completely rescaled by the disorder amplitude $\sigma$, as a function of the system size $N$, for different $\sigma$. (b) Proxy for the distance to amnesia, $1/\kappa$, as a function of the loading rate $c$, for different system size $N$. (c) Inverse of the rescaled amnesia rate completely rescaled by the system size $N$, as a function of the loading rate $c$, for different $N$.

## VI. DETAILS ABOUT THE AMNESIA PHASE DIAGRAM

In Fig. 4 of the main text, we present a phase diagram for the rescaled amnesia rate depending on the loading, the disorder and the system size. This phase diagram is built from the interpolation of the results obtained from simulations carried out with more than 400 different sets of parameters. In the movie 'phase_diagram.avi' (see snapshots in Fig.5) we rotate a 3D representation of these raw data.

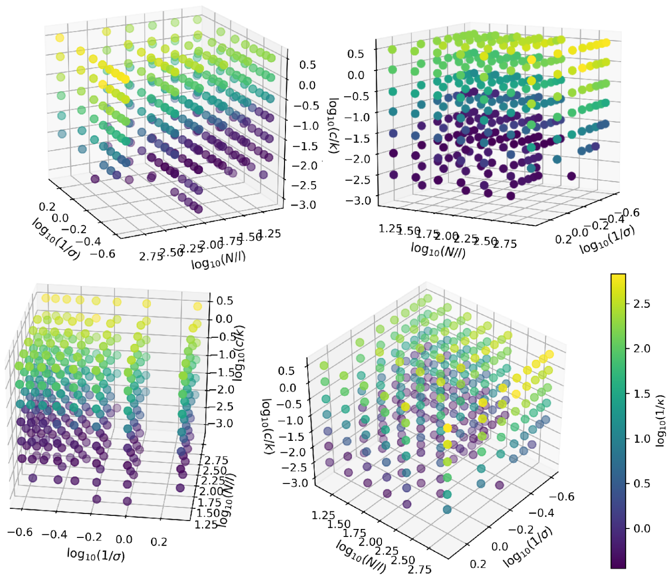


Figure 5. Snapshots of the movie presenting the raw data of the phase diagram: 'phase_diagram.avi'.

When building this phase diagram, we found in a marginal number of cases very small oscillations on two loops in the limit cycles. These oscillations happen very close to the numerical resolution, and more importantly they do not impact the amnesia rates that we report. These very rare cases occurred for small system size $N$, large disorder strength $\sigma$, and/or low speed loading $c$, in other words deep in the intermittent phase. A example is shown thereafter in Sec. VIII.

## VII. CONTINUOUS VERSUS INTERMITTENT VELOCITY DYNAMICS

In the main text, we identify two different amnesia regimes, namely, a regime **A** where the memory is extensive ($\kappa$ follows a well-defined scaling law) and a regime **B** where the amnesia rate $\kappa$ saturates. A phase diagram showing where these regimes are located in the parameter space has been built in Fig. 4 of the main text. We map both regimes with different dynamical behaviours already identified in [1, 4]: **A** corresponds with a continuous propagation of the front while **B** corresponds with an intermittent behaviour. To clarify this point, in Fig. 6 for 6 randomly peaked simulation points (3 in **A** and 3 in **B**), we both show their position in the phase diagram and their $\bar{v}(t)$ curves characterising their dynamical behaviour.

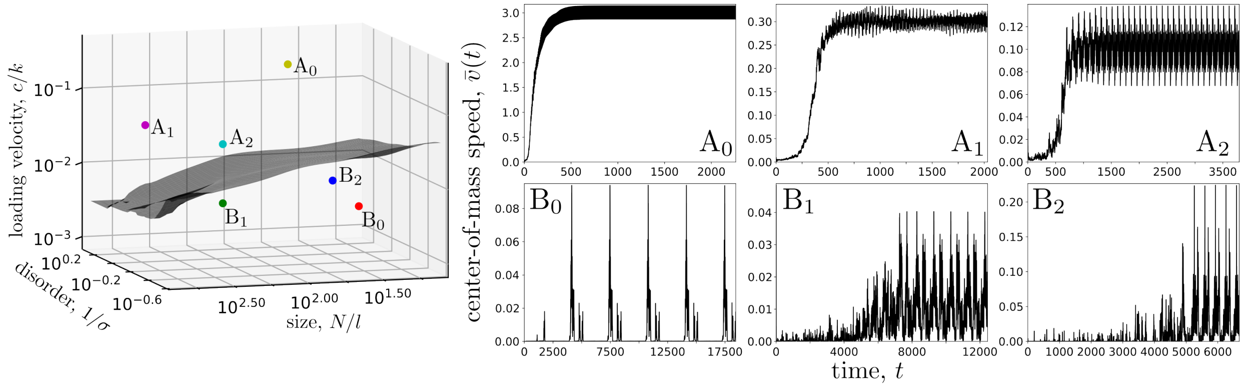


Figure 6. *Left:* repeated phase diagram from Fig. 4 of the main text with randomly peaked points above and below the surface separating both phases. *Right:* $\bar{v}(t)$ curves of the simulations corresponding to the points peaked in the phase diagram.

## VIII. TYPICAL CASE WITH PERIODIC LIMIT CASE

In very rare cases, for small system size $N$, large disorder amplitude, or low speed loading $c$, we observed, deep in the intermittent phase, very small oscillations on few loops in the limit cycles. This is reminiscent of what is sometimes observed in cyclically sheared amorphous systems. A more careful study of these systems (for which parameters they occur, what is their period...) is of great interest but is out of the scope of the current manuscript.

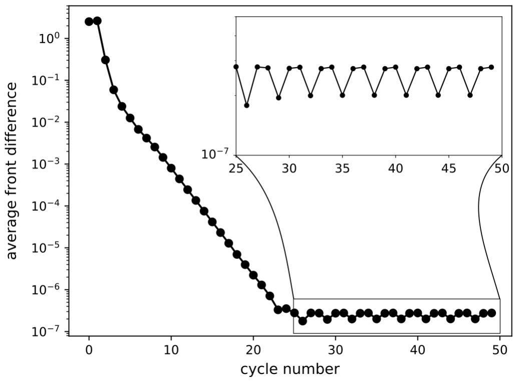


Figure 7. Exponential decay of the integrated profile difference $\Delta h_j$, plateauing in a cyclic manner. Parameters: $c = 3 \times 10^{-3}$, $k = 10^{-2}$, $\sigma = 4$, $N = 256$, $l = 10$.

[1] J. Barés, L. Barbier, and D. Bonamy. Crackling versus Continuumlike Dynamics in Brittle Failure. *Phys. Rev. Lett.* **111**, 054301 (2013).
[2] Jonathan Barés and Daniel Bonamy. Crack growth in heterogeneous brittle solids: intermittency, crackling and induced seismicity. *Philosophical Transactions of the Royal Society A: Mathematical, Physical and Engineering Sciences* **377**, 20170386 (2019).
[3] Jonathan Barés, Daniel Bonamy, and Alberto Rosso. Seismiclike organization of avalanches in a driven long-range elastic string as a paradigm of brittle cracks. *Phys. Rev. E* **100**, 023001 (2019).
[4] Jonathan Barés and Daniel Bonamy. Controlling crackling dynamics by triggering low-intensity avalanches. *Phys. Rev. E* **103**, 053001 (2021).
